# Supplementary material for: Holi-Spatial: Evolving Video Streams into Holistic 3D Spatial Intelligence
Source: arXiv:2603.07660 source file (2026-03-08)
Supplement: Supplementary file 1 [file 05_sft.tex]

\section{Can We Teach VLMs to Build and Leverage Spatial Representations?}
In the main paper, we demonstrated that prompting frozen VLMs with external scaffolds offers limited improvements. This highlighted a core limitation: the models themselves aren't effectively forming internal spatial representations or reasoning through space. To address this, we investigated whether supervised fine-tuning (SFT) could teach VLMs to build and leverage these spatial models internally. This section of the appendix provides further details on our SFT methodology, starting with the crucial step of data curation.

\subsection{Supervised Fine-Tuning Data Curation}
Effective SFT heavily relies on the quality and nature of the training data. To teach our VLMs the desired spatial reasoning capabilities, we meticulously curated two primary types of data: cognitive maps and free-form reasoning chains. These were designed to provide strong supervisory signals for the model to learn how to represent and reason about space.

\subsubsection{Cognitive Map Generation} \label{app_sec:sft_cogmap_gen}
As discussed in Section~\ref{app_sec:data_structure}, cognitive maps serve as 2D schematic representations of object layouts. For the SFT phase, we needed to generate ground truth cognitive maps that the VLM could learn to produce. Our approach to generating these maps was grounded in the object arrangement annotations described in Section~\ref{app_sec:mindcube_collection}. We aimed for representations that were not only accurate but also in a format that the VLM could feasibly learn to generate.

The generation process was automated via a script that processes input JSONL files, where each line item contains scene details including images and, crucially, \texttt{meta\_info} describing the objects, their potential orientations, and the camera viewpoint setup. For every item, the script first identifies its specific spatial arrangement "setting" (e.g., "around," "among," "translation," or "rotation") by parsing the item's unique ID. Based on this setting, dedicated functions apply a set of predefined rules and heuristics to determine the 2D coordinates (on a 10x10 grid) and facing directions for both the objects and the camera views.

For instance, in the "around" setting, objects (typically 2-4) are placed in a predetermined linear arrangement near the grid's center (e.g., at coordinates like [4,5], [5,5]), and camera views are positioned at cardinal directions relative to these objects, based on the specific camera angles pertinent to the question. In the "rotation" setting, the camera is fixed at the center ([5,5]), and its facing direction changes across views, while object positions are defined relative to the camera's current orientation. Similar rule-based placements are implemented for "among" (objects in a cross or T-shape with views from specific angles) and "translation" (objects arranged linearly to depict relationships like "on" or "down to") settings. Object orientations, if applicable, are also assigned based on the input \texttt{meta\_info}.

Finally, the generated layout of objects and views is formatted into a structured JSON string, representing the cognitive map. This JSON cogmap, along with templated instructional prompts (\texttt{cogmap\_input} for VLM input format guidance and \texttt{cogmap\_output} for VLM output task description), is added to the original data item. The overall generation logic is summarized in Algorithm~\ref{alg:cogmap_generation}.

\begin{algorithm}[htbp]
\caption{Cognitive Map Generation} \label{alg:cogmap_generation}
\begin{algorithmic}[1]
\Require Dataset $D$ containing items with spatial arrangement annotations
\Ensure Updated dataset with cognitive maps in JSON format

\ForAll{$item \in D$}
    \State $setting \gets$ Extract setting type from $item.id$
    \State Initialize empty cognitive map $cogmap$
    
    \Comment{Position objects and views based on setting type}
    \If{$setting = \text{``around''}$}
        \State Position 2-4 objects in a line with coordinates like [4,5], [5,5], etc.
        \State Place views at cardinal positions based on camera angles
    \ElsIf{$setting = \text{``among''}$}
        \State Place center object at [5,5] and surrounding objects at [5,8], [2,5], [5,2], [8,5]
        \State Position views based on specified camera angles
    \ElsIf{$setting = \text{``translation''}$}
        \State Position objects according to their spatial relationships (e.g., ``on'', ``down'')
        \State Place views to highlight these spatial relationships
    \ElsIf{$setting = \text{``rotation''}$}
        \State Arrange objects based on rotation type (clockwise, counterclockwise, etc.)
        \State Fix camera at [5,5] with varying facing directions
    \EndIf
    
    \Comment{Add orientation information where applicable}
    \ForAll{$object \in cogmap.objects$}
        \If{$object$ has orientation}
            \State Add facing direction (``up'', ``down'', ``left'', ``right'')
        \EndIf
    \EndFor
    
    \State Format $cogmap$ as structured JSON
    \State Add formatted cognitive map to $item$
\EndFor
\State \Return Updated dataset $D$
\end{algorithmic}
\end{algorithm}

\subsubsection{Free-Form Reasoning Generation} \label{app_sec:sft_ffr_gen}
While cognitive maps provide a structured, global understanding of the scene, effective spatial reasoning also involves a procedural, step-by-step thought process. To instill this capability in our VLMs, we generated a dataset of grounded free-form reasoning chains. These chains were designed to verbalize the mental simulation process required to answer the spatial questions in \name.

The generation of these reasoning chains was closely tied to the question-answer (QA) templates developed in Section 2. For each specific setting (e.g., rotation, among, around), we manually constructed reasoning chains following a consistent set of principles to ensure logical coherence and clear grounding in the provided visual information and the question asked.

The core principles guiding the generation of these reasoning chains were:
\begin{enumerate}[leftmargin=12pt, topsep=-1pt, itemsep=0pt]
    \item \textbf{Initial Scene Understanding.} The reasoning begins by processing each input image individually. This involves identifying key objects visible in that view and noting their explicit spatial relationships with other objects within that same view. This step emulates the initial perceptual intake a human might perform.
    \item \textbf{Cross-View Consistency and Environment Integration.} After individual view analysis, the reasoning emphasizes that although different images are provided, they all depict the \textit{same underlying spatial environment}. This is often achieved by identifying and highlighting an anchor object or a consistent set of objects that appear across multiple views, thereby helping to establish a unified mental model of the scene.
    \item \textbf{Question-Driven Inference.} With a foundational understanding of the scene established from the views, the subsequent steps in the reasoning chain are directly guided by the specifics of the question. This involves: (1) \textbf{Mental Simulation:} If the question involves a hypothetical change in viewpoint or a "what-if" scenario (e.g., "what if you turn left?"), the reasoning chain explicitly verbalizes this mental transformation. (2) \textbf{Perspective Taking:} If the question requires adopting a different perspective (e.g., "from the sofa's perspective"), the reasoning chain articulates this shift. (3) \textbf{Spatial Relationship Deduction:} The chain logically deduces the queried spatial relationship by integrating information from the relevant views, applying spatial concepts (like left-of, behind, further from), and referencing the established mental model of the scene.
\end{enumerate}

This structured approach to generating reasoning chains aimed to provide clear, step-by-step examples of spatial thought processes for the VLM to learn from. Figure~\ref{fig:reasoning_rotation},~\ref{fig:reasoning_among} and~\ref{fig:reasoning_around} show a template example combined with the filled case for \textsc{Rotation}, \textsc{Among}, \textsc{Around}, respectively.

\subsection{Detailed Experimental Setup} \label{app_sec:sft_exp_setup}

\begin{wraptable}{r}{0.5\textwidth}
\centering
\vspace{-1.5em} %
\caption{Training hyperparameters for SFT experiments with \modelname.}
\label{tab:sft_training_settings_appendix}
\begin{tabular}{ll}
\toprule
\textbf{Parameter}         & \textbf{Value}            \\
\midrule
Dataset size               & 10,000 QA pairs           \\
Epochs                     & 3                         \\
Learning rate              & 1e-5                      \\
Scheduler                  & Cosine                    \\
Fine-tuning type           & Full-parameter            \\
Batch Size       & 256 \\ 
GPUs used                  & 2 × NVIDIA H100  \\
Max image resolution       & 90,000 pixels             \\
Min image resolution       & 784 pixels                \\
Model Max Length           & 8192 tokens               \\
Weight Decay               & 0                         \\
Warmup Ratio               & 0.03                      \\
Max Grad Norm              & 1                         \\
Precision                  & BF16                      \\
Optimizer                  & AdamW      \\ %
\bottomrule
\end{tabular}
\vspace{-2ex} %
\end{wraptable}

In this section, we provide a more granular view of the experimental parameters employed during the Supervised Fine-Tuning (SFT) phase of our research. As stated in the main text, these experiments were designed to teach Vision-Language Models (VLMs) to build and leverage internal spatial representations. The base model for these SFT experiments was \modelname.

We utilized a consistent training script for all SFT experiments, ensuring comparability across different configurations. The primary variation across these runs was the specific dataset used (datasets variable in the script), corresponding to the different SFT task configurations discussed in Section 4.1, such as \texttt{Aug-CGMap-Out}. Other hyperparameters were kept constant to isolate the effects of the different training signals.

The core training hyperparameters are summarized in Table \ref{tab:sft_training_settings_appendix} and further detailed by the provided training script.

\begin{figure}[htbp]
    \centering
    \includegraphics[width=\linewidth]{figs/app_reasoning_exp_rotation.pdf}
    \caption{Example reasoning chain template for \textsc{Rotation}}
    \label{fig:reasoning_rotation}
\end{figure}
\begin{figure}[htbp]
    \centering
    \includegraphics[width=\linewidth]{figs/app_reasoning_exp_among.pdf}
    \caption{Example reasoning chain template for \textsc{Among}}
    \label{fig:reasoning_among}
\end{figure}

\begin{figure}[htbp]
    \centering
    \includegraphics[width=.92\linewidth]{figs/app_reasoning_exp_around.pdf}
    \caption{Example reasoning chain template for \textsc{Around}}
    \label{fig:reasoning_around}
    \vspace*{-1.5em}
\end{figure}

The training was conducted using a distributed setup managed by \texttt{torchrun} and leveraged DeepSpeed with a ZeRO Stage 3 optimization strategy for efficient full-parameter fine-tuning. Specifically, we set \texttt{NPROC\_PER\_NODE} to 2, utilizing two NVIDIA H100 GPUs, though the script template showed \texttt{CUDA\_VISIBLE\_DEVICES=0,1,2,3} and \texttt{NPROC\_PER\_NODE} defaulting to 4, our table and resource claims point to 2 GPUs being used for these runs. The \texttt{per\_device\_train\_batch\_size} was set to 4, and with \texttt{gradient\_accumulation\_steps} at 32, this resulted in an effective batch size of 256.

The learning rate was $1 \times 10^{-5}$ with a cosine learning rate scheduler and a warmup ratio of 0.03 over 3 training epochs. We enabled full fine-tuning of the vision encoder, MM-MLP, and the LLM components (\texttt{--tune\_mm\_vision True --tune\_mm\_mlp True --tune\_mm\_llm True}). The maximum sequence length for the model was set to 8192 tokens (\texttt{--model\_max\_length 8192}), and the maximum image input pixels were capped at 90,000 (\texttt{--max\_pixels 90000}), with a minimum of 784. Gradient checkpointing was enabled to manage memory usage (\texttt{--gradient\_checkpointing True}). Checkpoints were saved every 5 steps (\texttt{--save\_steps 5}), keeping a total of 12 checkpoints (\texttt{--save\_total\_limit 12}).

This consistent and robust experimental framework, detailed in Sections 3.1, 3.2, and herein, allowed for a fair comparison of the different SFT strategies aimed at improving the spatial reasoning capabilities of \modelname.

\subsection{VLM Response Examples After SFT for Configurations in  Section \ref{app_sec:example_configuration}}
\begin{tcolorbox}[colback=boxbackground, colframe=accentblue, 
title=Output for \texttt{Raw-QA}: Input Prompt Refer to \ref{app_sec:config_rawqa}, boxrule=0.5mm, width=\textwidth, arc=2mm, auto outer arc=true, breakable]
<answer>\textcolor{red}{\bf D. White headboard}</answer>
\end{tcolorbox}

\bigskip

\begin{tcolorbox}[colback=boxbackground, colframe=accentblue, 
title=Output for \texttt{Aug-CGMap-Out}: Input Prompt Refer to \ref{app_sec:config_ag_cgmap_out}, boxrule=0.5mm, width=\textwidth, arc=2mm, auto outer arc=true, breakable]
Based on my observation, the answer is:
\newline
<cogmap>
\begin{verbatim}
```json
{
  "objects": [
    {"name": "white jar", "position": [5, 5]},
    {"name": "bed sheet with a floral pattern", "position": [5, 8]},
    {"name": "white headboard", "position": [2, 5]},
    {"name": "clothes rack", "position": [5, 2]},
    {"name": "table with cups on it", "position": [8, 5]}
  ],
  "views": [
    {"name": "Image 1", "position": [5, 6], "facing": "up"},
    {"name": "Image 2", "position": [4, 5], "facing": "right"},
    {"name": "Image 3", "position": [5, 4], "facing": "down"},
    {"name": "Image 4", "position": [6, 5], "facing": "left"}
  ]
}
'''
\end{verbatim}
</cogmap>
<answer>\textcolor{mygreen}{\bf C. Bed sheet with a floral pattern}</answer>
\end{tcolorbox}

\bigskip

\begin{tcolorbox}[colback=boxbackground, colframe=accentblue, 
title=Output for \texttt{Plain-CGMap-Out}: Input Prompt Refer to \ref{app_sec:config_plain_cgmap_out}, boxrule=0.5mm, width=\textwidth, arc=2mm, auto outer arc=true, breakable]
Based on my observation, the answer is:
\newline
<cogmap>
\begin{verbatim}
```json
{
    "white jar": {"position": [5, 5]}, 
    "bed sheet with a floral pattern": {"position": [5, 8]}, 
    "white headboard": {"position": [2, 5]}, 
    "clothes rack": {"position": [5, 2]}, 
    "table with cups on it": {"position": [8, 5]}
}
'''
\end{verbatim}
</cogmap><answer>
\textcolor{red}{\bf B. Clothes rack}
</answer>
\end{tcolorbox}

\bigskip

\begin{tcolorbox}[colback=boxbackground, colframe=accentblue, 
title=Output for \texttt{FF-Rsn}: Input Prompt Refer to \ref{app_sec:config_ff_rsn}, boxrule=0.5mm, width=\textwidth, arc=2mm, auto outer arc=true, breakable]
<think>In this scene, I observe four images showing different perspectives. All images feature the white jar as the main object. In image 1, I can see white jar in front of the table with cups on it. In image 2, I can see white jar in front of the bed sheet with a floral pattern. In image 3, I can see white jar in front of the clothes rack. In image 4, I can see white jar in front of the white headboard. To identify the position change across views, I focus on the main object's angle variation. Then, I analyze the angles and relative positions of other objects on the platform to back up this observation. I understand that:  Image 1 is the initial view. Image 2 is captured after a 90-degree clockwise rotation from image 1. Image 3 is after another 90-degree clockwise rotation (180 degrees from image 1). Image 4 is after a further 90-degree clockwise rotation (270 degrees from image 1). Through analyzing these perspective changes, I can construct a complete spatial understanding: when I view bed sheet with a floral pattern behind white jar in the second view, it implies that in the first view, bed sheet with a floral pattern is on the right side of white jar. Similarly, when I see white headboard behind white jar in the fourth view, it indicates that in the first view, white headboard is on the left side of white jar. However, I am still uncertain about what lies behind me in the first view. Then, I recognize that I can examine the opposite view to find out. The opposite view of the fist view is the third view. As clothes rack is observed behind white jar in the third view, it means that in the first view, clothes rack is positioned behind me. This way, I can fully comprehend the spatial relationships of all objects in the entire scene. So, from the perspective of image 4: table with cups on it is to the right of white jar, bed sheet with a floral pattern is to my behind, clothes rack is to the left of white jar. So the answer is B. Clothes rack</think><answer>\textcolor{red}{\bf B. Clothes rack}</answer>
\end{tcolorbox}

\bigskip

\begin{tcolorbox}[colback=boxbackground, colframe=accentblue, 
title=Output for \texttt{Aug-CGMap-FFR-Out}: Input Prompt Refer to \ref{app_sec:config_ag_cgmap_ffr_out}, boxrule=0.5mm, width=\textwidth, arc=2mm, auto outer arc=true, breakable]
Based on my observation, the answer is:
\newline
<cogmap>
\newline
\begin{verbatim}
```json
{
  "objects": [
    {"name": "white jar", "position": [5, 5]},
    {"name": "bed sheet with a floral pattern", "position": [5, 8]},
    {"name": "white headboard", "position": [2, 5]},
    {"name": "clothes rack", "position": [5, 2]},
    {"name": "table with cups on it", "position": [8, 5]}
  ],
  "views": [
    {"name": "Image 1", "position": [5, 6], "facing": "up"},
    {"name": "Image 2", "position": [4, 5], "facing": "right"},
    {"name": "Image 3", "position": [5, 4], "facing": "down"},
    {"name": "Image 4", "position": [6, 5], "facing": "left"}
  ]
}
'''
\end{verbatim}
</cogmap>
<think>In this scene, I observe four images showing different perspectives. All images feature the white jar as the main object. In image 1, I can see white jar in front of the table with cups on it. In image 2, I can see white jar in front of the clothes rack. In image 3, I can see white jar in front of the bed sheet with a floral pattern. In image 4, I can see white jar in front of the white headboard. To identify the position change across views, I focus on the main object's angle variation. Then, I analyze the angles and relative positions of other objects on the platform to back up this observation. I understand that:  Image 1 is the initial view. Image 2 is captured after a 90-degree clockwise rotation from image 1. Image 3 is after another 90-degree clockwise rotation (180 degrees from image 1). Image 4 is after a further 90-degree clockwise rotation (270 degrees from image 1). Through analyzing these perspective changes, I can construct a complete spatial understanding: when I view clothes rack behind white jar in the second view, it implies that in the first view, clothes rack is on the right side of white jar. Similarly, when I see white headboard behind white jar in the fourth view, it indicates that in the first view, white headboard is on the left side of white jar. However, I am still uncertain about what lies behind me in the first view. Then, I recognize that I can examine the opposite view to find out. The opposite view of the fist view is the third view. As bed sheet with a floral pattern is observed behind white jar in the third view, it means that in the first view, bed sheet with a floral pattern is positioned behind me. This way, I can fully comprehend the spatial relationships of all objects in the entire scene. So, from the perspective of image 4: clothes rack is to the right of white jar, bed sheet with a floral pattern is to my behind, table with cups on it is to the left of white jar. So the answer is A. Table with cups on it.</think><answer>\textcolor{red}{\bf A. Table with cups on it}</answer>
\end{tcolorbox}

\bigskip

\begin{tcolorbox}[colback=boxbackground, colframe=accentblue, 
title=Output for \texttt{Plain-CGMap-FFR-Out}: Input Prompt Refer to \ref{app_sec:config_plain_cgmap_ffr_out}, boxrule=0.5mm, width=\textwidth, arc=2mm, auto outer arc=true, breakable]
Based on my observation, the answer is:
\newline
<cogmap>
\newline
\begin{verbatim}
```json
{
    "white jar": {"position": [5, 5]}, 
    "bed sheet with a floral pattern": {"position": [5, 8]}, 
    "white headboard": {"position": [2, 5]}, 
    "clothes rack": {"position": [5, 2]}, 
    "table with cups on it": {"position": [8, 5]}
}
'''
\end{verbatim}
</cogmap>
<think>In this scene, I observe four images showing different perspectives. All images feature the white jar as the main object. In image 1, I can see white jar in front of the table with cups on it. In image 2, I can see white jar in front of the clothes rack. In image 3, I can see white jar in front of the bed sheet with a floral pattern. In image 4, I can see white jar in front of the white headboard. To identify the position change across views, I focus on the main object's angle variation. Then, I analyze the angles and relative positions of other objects on the platform to back up this observation. I understand that:  Image 1 is the initial view. Image 2 is captured after a 90-degree clockwise rotation from image 1. Image 3 is after another 90-degree clockwise rotation (180 degrees from image 1). Image 4 is after a further 90-degree clockwise rotation (270 degrees from image 1). Through analyzing these perspective changes, I can construct a complete spatial understanding: when I view clothes rack behind white jar in the second view, it implies that in the first view, clothes rack is on the right side of white jar. Similarly, when I see white headboard behind white jar in the fourth view, it indicates that in the first view, white headboard is on the left side of white jar. However, I am still uncertain about what lies behind me in the first view. Then, I recognize that I can examine the opposite view to find out. The opposite view of the fist view is the third view. As bed sheet with a floral pattern is observed behind white jar in the third view, it means that in the first view, bed sheet with a floral pattern is positioned behind me. This way, I can fully comprehend the spatial relationships of all objects in the entire scene. So, from the perspective of image 4: clothes rack is to the right of white jar, bed sheet with a floral pattern is to my behind, table with cups on it is to the left of white jar. So the answer is A. Table with cups on it.</think><answer>\textcolor{red}{\bf A. Table with cups on it}</answer>
\end{tcolorbox}

\subsection{Detailed Graph Metric Results for SFT Graph-Related Experiments}

This section provides a detailed look at the Supervised Fine-Tuning (SFT) training dynamics to support the main paper's conclusions. The figures below plot key metrics over training steps for four map-generation settings. A comparative analysis highlights that jointly training map generation and reasoning is the most effective strategy.

When training on map generation alone, as in the \texttt{Plain-CGMap-Out} and \texttt{Aug-CGMap-Out} settings, the graph quality metrics show rapid convergence. However, the final QA accuracy is limited, reaching 54.38\% for \texttt{Plain-CGMap-Out} and 54.19\% for \texttt{Aug-CGMap-Out}.

In contrast, the joint training approaches (\texttt{Plain-CGMap-FFR-Out} and \texttt{Aug-CGMap-FFR-Out}), despite a slower initial convergence on graph quality metrics, ultimately achieve far superior performance in task accuracy. The \texttt{Plain-CGMap-FFR-Out} setting proves to be the most effective, reaching a QA Accuracy of 60.00\%. The \texttt{Aug-CGMap-FFR-Out} setting also yields strong results, with QA accuracy climbing to about 65\%. This demonstrates the superiority of joint training for achieving high performance in both the final task accuracy and the quality of the generated spatial representations.

\begin{figure}[!ht]
    \centering
    \includegraphics[width=\linewidth]{figs/app_sft_line_2.pdf}
    \caption{Training dynamics for the \texttt{Aug-CGMap-Out} setting.}
    \label{fig:sft-aug-cgmap-out}
\end{figure}

\begin{figure}[!ht]
    \centering
    \includegraphics[width=\linewidth]{figs/app_sft_line_3.pdf}
    \caption{Training dynamics for the \texttt{Plain-CGMap-Out} setting.}
    \label{fig:sft-plain-cgmap-out}
\end{figure}

\begin{figure}[!ht]
    \centering
    \includegraphics[width=\linewidth]{figs/app_sft_line_1.pdf}
    \caption{Training dynamics for the \texttt{Aug-CGMap-FFR-Out} setting.}
    \label{fig:sft-aug-cgmap-ffr-out}
\end{figure}

\begin{figure}[!ht]
    \centering
    \includegraphics[width=\linewidth]{figs/app_sft_line_1.pdf}
    \caption{Training dynamics for the \texttt{Plain-CGMap-FFR-Out} setting, showing superior final performance.}
    \label{fig:sft-plain-cgmap-ffr-out}
\end{figure}

\subsection{Which Part of VLM is the Bottleneck for Spatial Understanding?}

To develop more efficient fine-tuning strategies, it is crucial to understand which component of a Vision-Language Model (VLM)---the vision encoder responsible for perception or the Large Language Model (LLM) responsible for reasoning---presents the primary bottleneck for spatial understanding. To investigate this, we conduct a bottleneck analysis by selectively fine-tuning different parts of the VLM and observing the impact on performance.

We evaluate four distinct training configurations on the \texttt{Raw-QA} task, with results captured at an early stage of training (step 57) to assess the initial learning dynamics. The configurations are: (1) the baseline performance of the pre-trained model without any fine-tuning; (2) fine-tuning only the vision encoder while keeping the LLM frozen; (3) fine-tuning only the LLM while keeping the vision encoder frozen; and (4) the standard approach of fine-tuning all parts of the model.

\begin{table}[htbp]
\centering
\caption{VLM Training Bottleneck Analysis (Step=57, in \%). Performance is measured on the \namesub benchmark under the Raw-QA setting.}
\label{tab:vlm_bottleneck}
\vspace{1.5em}
\begin{tabular}{lcccc}
\toprule
\textbf{Training Method} & \textbf{Overall} & \textbf{Rotation} & \textbf{Among} & \textbf{Around} \\
\midrule
Raw-QA (no fine-tuning) & 37.81 & 34.00 & 36.00 & 45.20 \\
Freeze LLM (Vision Encoder Only) & 37.81 & 30.50 & 37.00 & 45.60 \\
Freeze Vision Encoder (LLM Only) & 51.43 & 34.00 & 50.00 & 68.80 \\
Tune All Parts & 52.28 & 34.50 & 52.50 & 66.00 \\
\bottomrule
\end{tabular}
\end{table}

The results, presented in Table~\ref{tab:vlm_bottleneck}, offer several key insights. First, there is a dramatic performance leap from the no-fine-tuning baseline (37.81\% overall), but only when the language model is trained. Methods involving LLM fine-tuning achieve over 51\% accuracy, underscoring the necessity of adapting the model's reasoning capabilities.

Most strikingly, the performance bottleneck is almost exclusively concentrated in the LLM. Tuning only the LLM (\texttt{Freeze Vision Encoder}) yields an overall accuracy of 51.43\%, capturing nearly the full performance gain of end-to-end fine-tuning (52.28\%). In stark contrast, tuning only the vision encoder (\texttt{Freeze LLM}) provides no improvement whatsoever over the baseline (37.81\%). This indicates that the bottleneck is not shared between modules. For this spatial task, adapting the model's language-based reasoning is critical, while adapting its visual perception is surprisingly ineffective.

Intriguingly, the fact that fine-tuning only the vision encoder fails to improve performance is in itself a significant finding. A possible explanation is that the pre-trained visual features are already sufficient to extract the necessary objects and their properties. The core challenge of the task seems to lie not in \emph{what} is seen, but in \emph{how to reason} about the spatial relationships across a series of views—a task primarily handled by the LLM. In conclusion, our analysis suggests that the most significant gains come from adapting the reasoning module. For efficient tuning, freezing the vision encoder and focusing solely on the LLM proves to be a highly effective strategy, achieving nearly top-tier performance at a fraction of the computational cost.

\subsection{Branching from \texttt{Raw-QA} SFT Checkpoint}

In our main experiments, we fine-tuned the model for each specific task format starting from the base pre-trained VLM. A natural question arises: can a curriculum-based SFT approach further improve performance? Specifically, we investigate whether first fine-tuning the model on the simplest task format---`Raw-QA`, which only requires outputting the final answer---can establish a better foundation for learning to leverage more complex reasoning formats.

To test this hypothesis, we conducted a set of branching experiments. We took the checkpoint from the model fully fine-tuned on the `Raw-QA` task. Then, we used this specialized checkpoint as the initial weights for further fine-tuning on other scaffolding tasks, namely \texttt{Aug-CGMap-In}, \texttt{FF Rsn}, and \texttt{Aug-CGMap-FFR-Out}. It is important to note that during this second stage of fine-tuning, the model's output for all tasks was still constrained to be only the final answer option. This setup allows us to isolate the effect of the cognitive scaffolds on the model's internal reasoning process, rather than its ability to generate complex text.

The results, presented in Table~\ref{tab:sft_from_rawqa}, show a consistent and notable improvement across all branched tasks compared to their counterparts trained from scratch. 
For example, both \texttt{Aug-CGMap-In} and \texttt{Aug-CGMap-FFR-Out} reach an impressive overall accuracy of 49.00\%. Even the \texttt{FF Rsn} method benefits from this two-stage approach, with its overall accuracy rising to 46.82\%. These findings suggest that a two-stage SFT strategy is highly effective. By first grounding the model in the fundamental objective of the task (i.e., finding the correct answer) and then teaching it to process and leverage more complex cognitive scaffolds, we can achieve superior spatial reasoning performance. This indicates that the model, once primed for the core task, becomes more adept at utilizing the provided spatial context, even if it does not explicitly generate the reasoning chain or cognitive map.

\begin{table}[h!]
\centering
\caption{Performance of various methods after being fine-tuned from a \texttt{Raw-QA} SFT checkpoint. This two-stage training approach led to performance gains across all methods. All accuracies are reported as percentages (\%).}
\label{tab:sft_from_rawqa}
\vspace{1.5em}
\begin{tabular}{lcccc}
\toprule
\textbf{Method} & \textbf{Overall} & \textbf{Rotation} & \textbf{Among} & \textbf{Around} \\
\midrule
\texttt{Raw-QA}                  & 46.36 & 33.50 & 51.20 & 46.75 \\
\texttt{Aug-CGMap-In}            & 49.00 & 35.50 & 53.20 & 50.50 \\
\texttt{FF Rsn}                  & 46.82 & 37.00 & 50.60 & 47.00 \\
\texttt{Aug-CGMap-FFR-Out}       & 49.00 & 37.00 & 53.20 & 49.75 \\
\bottomrule
\end{tabular}
\end{table}
