# Supplementary material for: Holi-Spatial: Evolving Video Streams into Holistic 3D Spatial Intelligence
Source: arXiv:2603.07660 source file (2026-03-08)
Supplement: Supplementary file 2 [file 06_rl.tex]

\section{Can Reinforcement Learning Further Refine Spatial Thought Processes?}
As discussed in the main paper, while Supervised Fine-Tuning (SFT) establishes a strong foundation for spatial reasoning, reinforcement learning (RL) presents an avenue for further optimizing spatial thought processes through outcome-driven feedback. The core inquiry is whether guiding VLMs with rewards can lead to the development of more precise spatial mental models and enhanced reasoning capabilities. This section of the appendix provides a more detailed exposition of the experimental setup employed for the RL phase of our research. Additionally, we present case studies to offer qualitative insights into how RL refines the models' spatial representations and reasoning chains.

\subsection{Detailed Experimental Setup} \label{app_sec:rl_exp_setup}
For the reinforcement learning (RL) phase of our research, we employed the VAGEN framework. The core policy optimization algorithm used was Group Relative Policy Optimization (GRPO). To ensure consistency and allow for direct comparison with earlier stages of our work, key components from the Supervised Fine-Tuning (SFT) experiments were retained. Specifically, the base Vision-Language Model (VLM) for all RL configurations was Qwen2.5-VL-3B-Instruct, and evaluations were performed on the MINDCUBE-TINY benchmark. All previously established evaluation metrics were also retained.

In consideration of computational costs, each distinct RL configuration was trained for a duration of 0.5 epoch. The primary hyperparameters governing the RL training process were set as follows:
\begin{itemize}[leftmargin=12pt, topsep=-1pt, itemsep=0pt]
    \item \textbf{Training Batch Size:} 32
    \item \textbf{Maximum Prompt Length:} 1024 tokens
    \item \textbf{Maximum Response Length:} 512 tokens
    \item \textbf{Actor Learning Rate:} $1 \times 10^{-6}$
    \item \textbf{Critic Learning Rate:} $1 \times 10^{-5}$
    \item \textbf{Number of Trajectories per Rollout:} 8
    \item \textbf{Maximum Turns per Trajectory:} 1
\end{itemize}

As detailed in Section 5.1 of the main paper, we investigated three RL task configurations:
\begin{enumerate}[leftmargin=12pt, topsep=-1pt, itemsep=0pt]
    \item \textbf{RL-FF-Rsn (from scratch):} The Qwen2.5-VL-3B-Instruct model was trained to generate free-form reasoning chains without prior SFT for this specific task format.
    \item \textbf{RL-Aug-CGMap-FFR-Out (from scratch):} The model was trained to jointly produce augmented cognitive maps and associated free-form reasoning, also starting from the base pre-trained VLM.
    \item \textbf{RL-Aug-CGMap-FFR-Out (from SFT):} For this configuration, the RL training was initialized using the weights from the strongest performing SFT checkpoint, specifically the Aug-CGMap-FFR-Out SFT model.
\end{enumerate}

The reward function was designed to be sparse yet directly indicative of desired behaviors. A reward of +1 was assigned if the model's output was structurally valid (e.g., the generated cognitive map adhered to the predefined schema). A more significant reward of +5 was given if the model provided the correct final answer to the spatial reasoning question. This dual-component reward was intended to steer the learning process towards generating both well-formed intermediate spatial representations and achieving high end-task accuracy.

\subsection{VLM Response Examples After RL for Configurations in  Section \ref{app_sec:example_configuration}}

\begin{tcolorbox}[colback=boxbackground, colframe=accentblue, 
title=Output for \texttt{FF-Rsn}: Input Prompt Refer to \ref{app_sec:config_ff_rsn}, boxrule=0.5mm, width=\textwidth, arc=2mm, auto outer arc=true, breakable]
<think>From image 4, the white jar is positioned on a surface with a floral-patterned bed sheet. To the left of the jar, there is a table with a pink tablecloth featuring heart shapes and a Hello Kitty design. There are also cups on the table. Therefore, the object to the left of the white jar is the table with the cups.</think><answer>\textcolor{red}{\bf A. Table with cups on it}</answer>
\end{tcolorbox}

\bigskip

\begin{tcolorbox}[colback=boxbackground, colframe=accentblue, 
title=Output for \texttt{RL-Aug-CGMap-FFR-Out (from scratch)}: Input Prompt Refer to \ref{app_sec:config_ag_cgmap_ffr_out}, boxrule=0.5mm, width=\textwidth, arc=2mm, auto outer arc=true, breakable]
<cogmap>
\begin{verbatim}
{
  "objects": [
    {"name": "white jar", "position": [265, 436], "facing": "left"}
  ],
  "views": [
    {"name": "View/Image 1", "position": [265, 436], 
      "facing": "left"},
    {"name": "View/Image 2", "position": [265, 436], 
      "facing": "left"},
    {"name": "View/Image 3", "position": [265, 436], 
      "facing": "left"},
    {"name": "View/Image 4", "position": [265, 436], 
      "facing": "left"}
  ]
}
\end{verbatim}
<Your cognitive map>
</cogmap>
\newline
<think>
The white jar is located in the center of the 10x10 grid, facing to the left. The clothes rack is to the left of the white jar, as seen in the image 2 view. The bed sheet with a floral pattern is located to the right of the white jar, as seen in the image 1 view. The white headboard is not visible in any of the provided images.
\newline
Based on the provided images, the white jar is located in the center of the 10x10 grid, facing to the left. The clothes rack is to the left of the white jar, as seen in the image 2 view. The bed sheet with a floral pattern is located to the right of the white jar, as seen in the image 1 view. The white headboard is not visible in any of the provided images.</think><answer>\textcolor{red}{\bf A. Table with cups on it}.</answer>
\end{tcolorbox}

\bigskip

\begin{tcolorbox}[colback=boxbackground, colframe=accentblue, 
title=Output for \texttt{RL-Aug-CGMap-FFR-Out (from SFT)}: Input Prompt Refer to \ref{app_sec:config_ag_cgmap_ffr_out}, boxrule=0.5mm, width=\textwidth, arc=2mm, auto outer arc=true, breakable]
Based on my observation, the answer is:
\newline
<cogmap>
\begin{verbatim}
```json
{
  "objects": [
    {"name": "white jar", "position": [5, 5]},
    {"name": "bed sheet with a floral pattern", "position": [5, 8]},
    {"name": "white headboard", "position": [2, 5]},
    {"name": "clothes rack", "position": [5, 2]},
    {"name": "table with cups on it", "position": [8, 5]}
  ],
  "views": [
    {"name": "Image 1", "position": [5, 6], "facing": "up"},
    {"name": "Image 2", "position": [4, 5], "facing": "right"},
    {"name": "Image 3", "position": [5, 4], "facing": "down"},
    {"name": "Image 4", "position": [6, 5], "facing": "left"}
  ]
}
'''
\end{verbatim}
</cogmap>
<think>
In this scene, I observe four images showing different perspectives. All images feature the white jar as the main object. In image 1, I can see white jar in front of the clothes rack. In image 2, I can see white jar in front of the table with cups on it. In image 3, I can see white jar in front of the bed sheet with a floral pattern. In image 4, I can see white jar in front of the white headboard. To identify the position change across views, I focus on the main object's angle variation. Then, I analyze the angles and relative positions of other objects on the platform to back up this observation. I understand that:  Image 1 is the initial view. Image 2 is captured after a 90-degree clockwise rotation from image 1. Image 3 is after another 90-degree clockwise rotation (180 degrees from image 1). Image 4 is after a further 90-degree clockwise rotation (270 degrees from image 1). Through analyzing these perspective changes, I can construct a complete spatial understanding: when I view table with cups on it behind white jar in the second view, it implies that in the first view, table with cups on it is on the right side of white jar. Similarly, when I see white headboard behind white jar in the fourth view, it indicates that in the first view, white headboard is on the left side of white jar. However, I am still uncertain about what lies behind me in the first view. Then, I recognize that I can examine the opposite view to find out. The opposite view of the fist view is the third view. As bed sheet with a floral pattern is observed behind white jar in the third view, it means that in the first view, bed sheet with a floral pattern is positioned behind me. This way, I can fully comprehend the spatial relationships of all objects in the entire scene. So, from the perspective of image 4: clothes rack is to the right of white jar, table with cups on it is to my behind, bed sheet with a floral pattern is to the left of white jar. So the answer is C. Bed sheet with a floral pattern.</think>
<answer>\textcolor{mygreen}{\bf C. Bed sheet with a floral pattern}</answer>
\end{tcolorbox}
