# Supplementary material for: Holi-Spatial: Evolving Video Streams into Holistic 3D Spatial Intelligence
Source: arXiv:2603.07660 source file (2026-03-08)
Supplement: Supplementary file 3 [file 07_aabb.tex]

\section{Floor-aligned OBB Post-processing}
\label{app:floor_aligned_obb}

As described in the main text, Holi-Spatial first lifts 2D instance masks into 3D by back-projecting pixels using rendered depth and camera intrinsics, and then estimates an oriented bounding box (OBB) from the resulting instance point set to form initial 3D proposals.
While these raw OBBs already provide a compact geometric proxy, they may exhibit inconsistent roll/pitch across instances due to residual depth noise, partial observations, and view-dependent missing geometry, which in turn hurts the stability of downstream multi-view merging (e.g., IoU-based consolidation) and subsequent verification. 
To improve global consistency, we apply an additional floor-alignment post-processing module to refine the predicted instance OBBs (Fig.~\ref{fig:floor_aligned_obb_pipeline}).

\paragraph{Stage 1: Floor detector and reference axis definition.}
Given the set of input instance OBBs, we first select a floor candidate by choosing the OBB with the maximum volume (a strong prior in indoor scenes where the floor plane spans the largest extent). If this heuristic fails (e.g., floor is fragmented or missing), we fall back to searching other dominant planar structures such as wall/ceiling. From the selected reference OBB, we infer the global up-axis via a lightweight heuristic, which defines a consistent gravity-aligned coordinate frame for subsequent refinement.

\paragraph{Stage 2: Per-object OBB re-alignment and extent update.}
For each instance OBB, we iteratively re-orient the box to align its vertical axis with the estimated up-axis, while keeping yaw changes minimal (yaw-lock) to preserve the object’s azimuthal orientation. When the heuristic alignment is ambiguous, we optionally invoke a PCA-based fallback on the instance point set to obtain a stable principal direction. After re-orientation, we update the box extents using either a \emph{keep} policy (preserve original size) or an \emph{enclose} policy (tighten/expand to enclose the rotated support), ensuring the final OBB remains a valid enclosure of the underlying instance geometry.

\paragraph{Stage 3: Finalization.}
We perform a validation check (e.g., sanity constraints on axis orthogonality, extent positivity, and consistency with the inferred gravity direction). Boxes failing the check are reverted to their pre-alignment state. The output is a set of floor-aligned OBBs that are more consistent across instances and scenes, which empirically benefits later steps that rely on geometric agreement between proposals.

\begin{figure}[t]
    \centering
    \includegraphics[width=\linewidth]{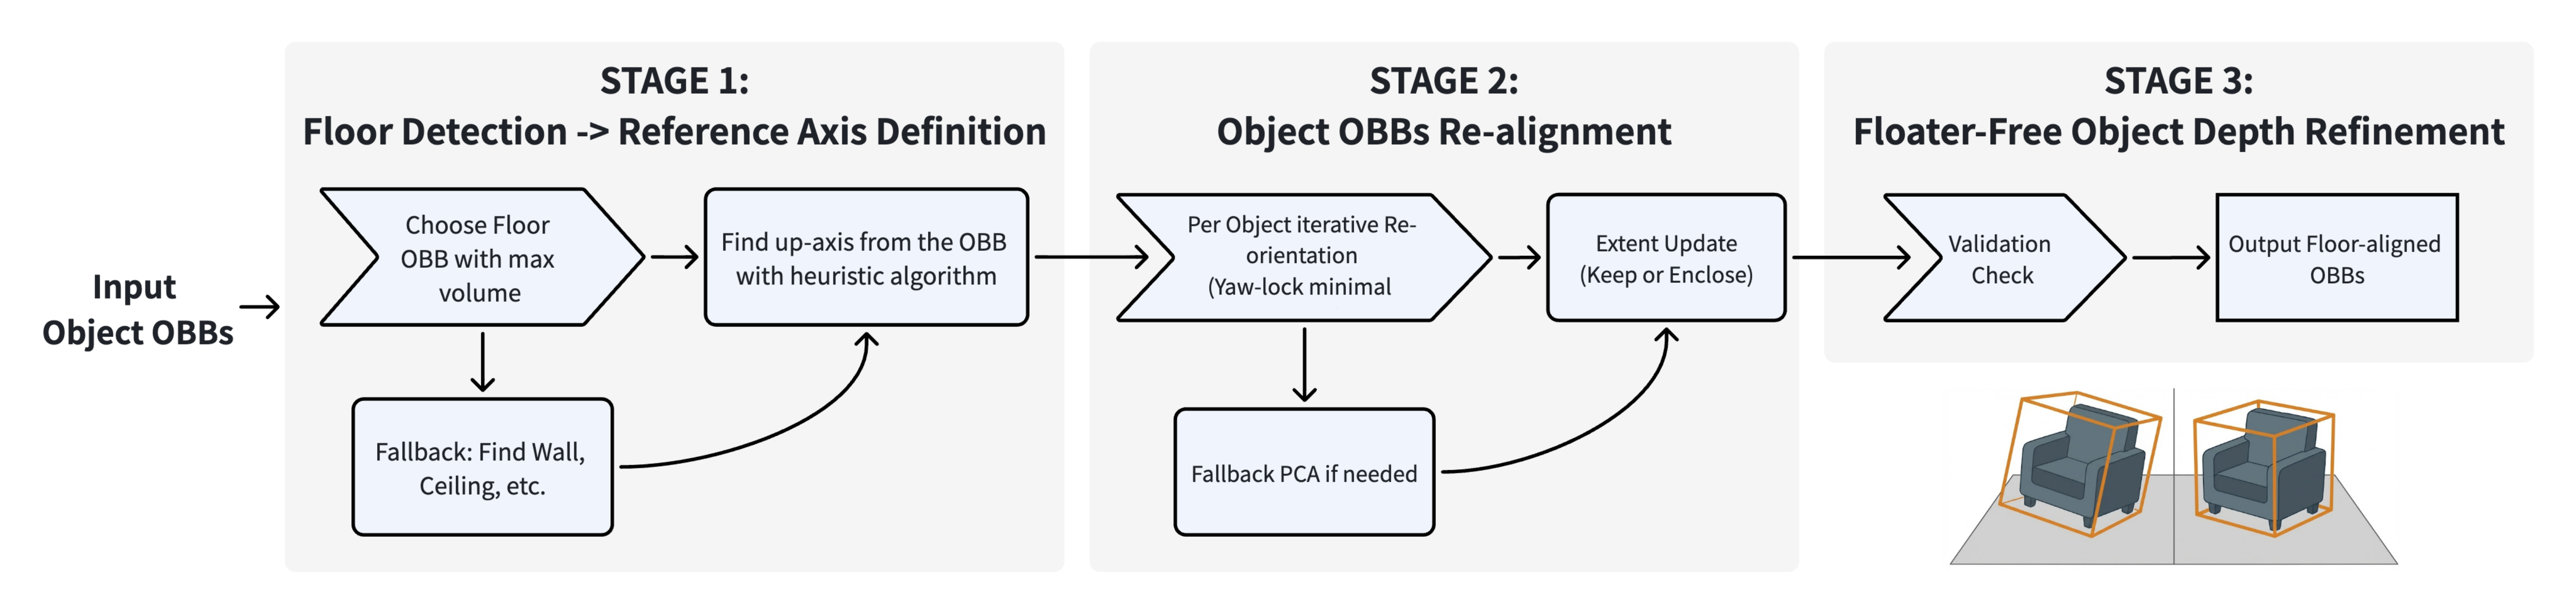}
    \caption{\textbf{Floor-aligned OBB post-processing pipeline.}
    Starting from the input instance OBBs produced after 2D-to-3D lifting and initial OBB estimation, we (1) detect a floor (or fallback planar structure) to infer a global up-axis, (2) re-align each instance OBB under a yaw-lock constraint with optional PCA fallback and update extents, and (3) apply a validation check to output gravity-/floor-consistent OBBs for downstream scene-level refinement.}
    \label{fig:floor_aligned_obb_pipeline}
\end{figure}
